# Supplementary material for: Activity gradients in two- and three-dimensional active nematics
Source: arXiv:2206.06499 ancillary file (2022-06-13)
Supplement: Supplementary file 1 [file SI.pdf]

# Supplementary information: Activity gradients in two- and three-dimensional active nematics


Liam J. Ruske and Julia M. Yeomans
*Rudolf Peierls Centre For Theoretical Physics, University of Oxford, Parks Road, Oxford OX1 3PU, UK*

(Dated: June 13, 2022)

## I. NUMERICAL IMPLEMENTATION

### A. Fluid simulation

In this work we use a finite-difference method to solve the equation of motion of the $Q$-tensor eq. (1), and a lattice Boltzmann algorithm to solve the fluid equations of motion eq. (3) [1–3]. The viscous and elastic contributions to the stress tensor in eq. (3) are

$$\Pi^{visc} = 2\eta\mathbf{D} , \tag{1}$$

$$\Pi^{el} = -p\mathbf{I} + \mathbf{QH} - \mathbf{HQ} - \nabla\mathbf{Q}\left(\frac{\partial f}{\partial(\nabla\mathbf{Q})}\right) , \tag{2}$$

where $D_{ij} = (\partial_j u_i + \partial_i u_j)/2$ is the symmetric part of the velocity gradient tensor.

Simulations were performed on 2D and 3D lattices of size $180 \times 90$ and $60 \times 60 \times 60$, respectively, and discrete space and time steps were chosen as unity. We used periodic boundary conditions for the simulation box and the system was initialized as $\mathbf{u} = \mathbf{0}$, $S = 0.3$ and random director field $\mathbf{n}$. We used the following parameter values unless otherwise stated: $\lambda = 30$, $K_{el} = 0.12$, $\zeta_{max} = 0.08$, $A = 0.08$, $B = -4.3$, $C = 4.3$, $\Gamma = 0.34$, fluid density $\rho = 1$, bulk pressure $p = 0.25$ and viscosity $\eta = 2/3$ in lattice-Boltzmann units.

### B. Defect tracking and polarization

To detect defect positions on a 2D or 3D grid we use Zapotoky's defect-finding algorithm [4], which we used previously to detect disclination lines in active nematic droplets [5]. In two dimensions, this algorithm checks if a defect is located at the intersection of four lattice sites forming a $2 \times 2$ square. In three-dimensional systems, disclination lines are found by repeating the two-dimensional square scan along all three coordinate axis [6]. The twist-angle $|\cos(\beta)|$ of a disclination is calculated using the local line tangent $\mathbf{t}$ and rotation vector $\Omega$. The latter is calculated by taking the cross product of each pair of directors around the disclination core. To distinguish whether $0 > \beta > \pi/2$ or $\pi/2 < \beta < \pi$, we calculate the saddle-splay energy $\bar{f}_{24} = \nabla \cdot [(\mathbf{n} \cdot \nabla)\mathbf{n} - \mathbf{n}(\nabla \cdot \mathbf{n})]$, which is negative for a $\beta > \pi/2$ disclination line segment and positive for a $\beta < \pi/2$ segment [7]. We classified disclination line segments as twist defects if $-0.1 < \cos(\beta) < 0.1$ and as $+1/2$ or $-1/2$ wedge-type defects if $\cos(\beta) < -0.8$ or $\cos(\beta) > 0.8$, respectively.

### C. Torque calculation

To calculate active and elastic torques on defects, we first obtain the hydrodynamical forces $F_i$ from the respective stress tensor

$$F_i = \partial_j \Pi_{ij} , \tag{3}$$

where $\Pi_{ij} = \Pi_{ij}^{el}$ for elastic forces and $\Pi_{ij} = \Pi_{ij}^{act}$ for active forces. The torque $\mathbf{\Gamma}$ on defects is then calculated by integrating forces in the vicinity of defects,

$$\Gamma_i = \int \epsilon_{ijk} F_j r_k \, dV , \tag{4}$$

where the origin of coordinate system $r_k$ is located at the centre of defects. We perform the integration over a circular domain $r < r_c$ around the defect core, where the cut-off radius $r_c$ is chosen as the average separation between defects.

In 3D systems, active and elastic torques acting on disclination line segments are calculated by integrating forces within a cylindrical domain which extends along the line tangent of disclination lines (see Fig. S6, Fig. 5 b).


[1] D. Marenduzzo, E. Orlandini, M. E. Cates, and J. M. Yeomans, Physical Review E **76**, 031921 (2007).
[2] P.-G. De Gennes and J. Prost, *The Physics of Liquid Crystals*, vol. 83 (Oxford university press, 1993).
[3] A. N. Beris and B. J. Edwards, *Thermodynamics of flowing systems with internal microstructure*, Oxford engineering science series ; 36 (Oxford University Press, New York ; Oxford, 1994), ISBN 9780195076943.
[4] M. Zapotocky, P. M. Goldbart, and N. Goldenfeld, Physical Review E **51**, 1216 (1995).
[5] L. J. Ruske and J. M. Yeomans, Physical Review X **11**, 021001 (2021).
[6] J. Hobdell and A. Windle, Liquid Crystals **23**, 157 (1997).
[7] L. Tran, M. O. Lavrentovich, D. A. Beller, N. Li, K. J. Stebe, and R. D. Kamien, Proceedings of the National Academy of Sciences **113**, 7106 (2016).

## II. SUPPLEMENTARY FIGURES

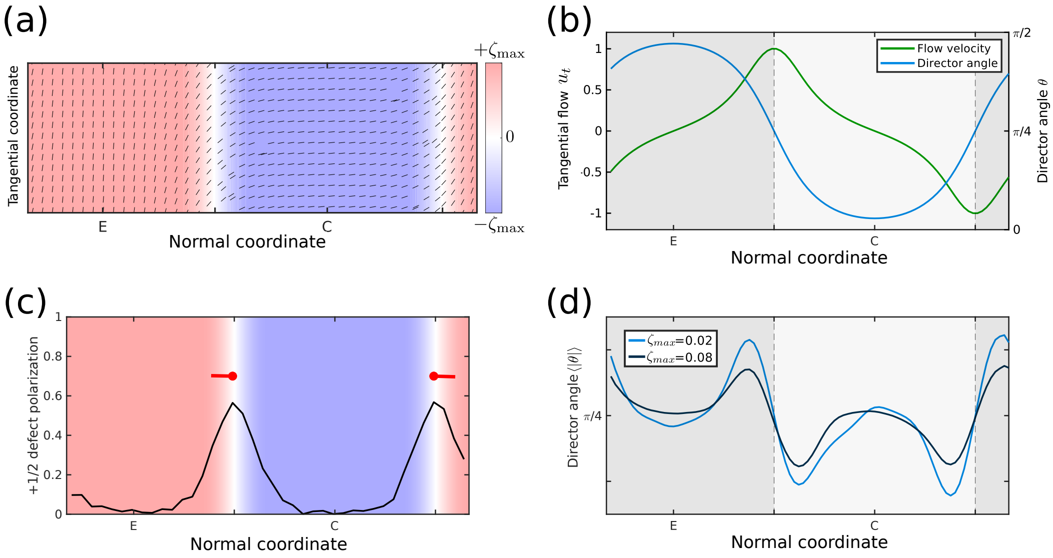


FIG. S1: (a) Sharp activity interfaces in 2D systems give rise to qualitatively similar dynamics in the laminar regime as sinusoidal activity variations. (b) Tangential flows are more strongly confined to the interface giving rise to a slightly different director profile. (c) In the turbulent state +1/2 defects show strong polarization at interfaces, which vanishes in contractile and extensile bulk regions. (d) As expected for isotropic active turbulence, in bulk regions there is no average alignment of the director field , $\langle|\theta|\rangle = \pi/4$. Close to activity interfaces there is a finite average alignment, which decreases with increasing active stress $\zeta_{max}$.

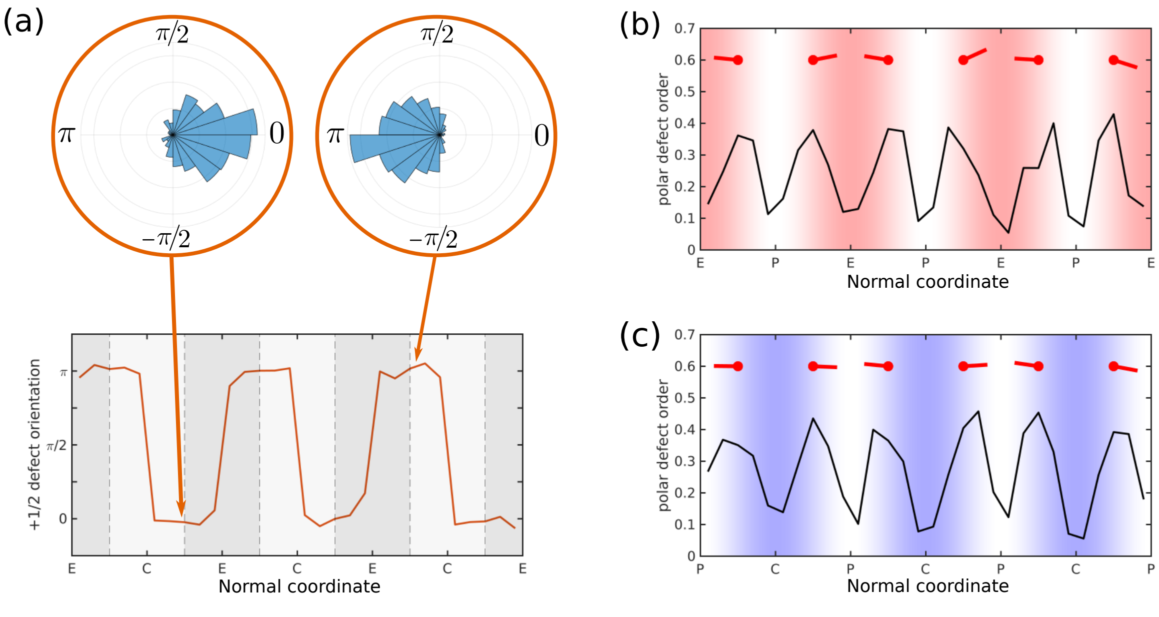


FIG. S2: (a) Defect polarization magnitude and direction are calculated based on the time-averaged distribution of defect orientations $\mathbf{p}$. (b,c) 2D systems with extensile-passive domains (b) or contractile-passive domains (c) with activity profiles $\zeta(\mathbf{x}) = \zeta_{max}(\cos(\mathbf{k}\cdot\mathbf{x}) \pm 1)$ show the same defect polarization as observed in extensile-contractile systems but the magnitude of defect polarization is slightly lower.

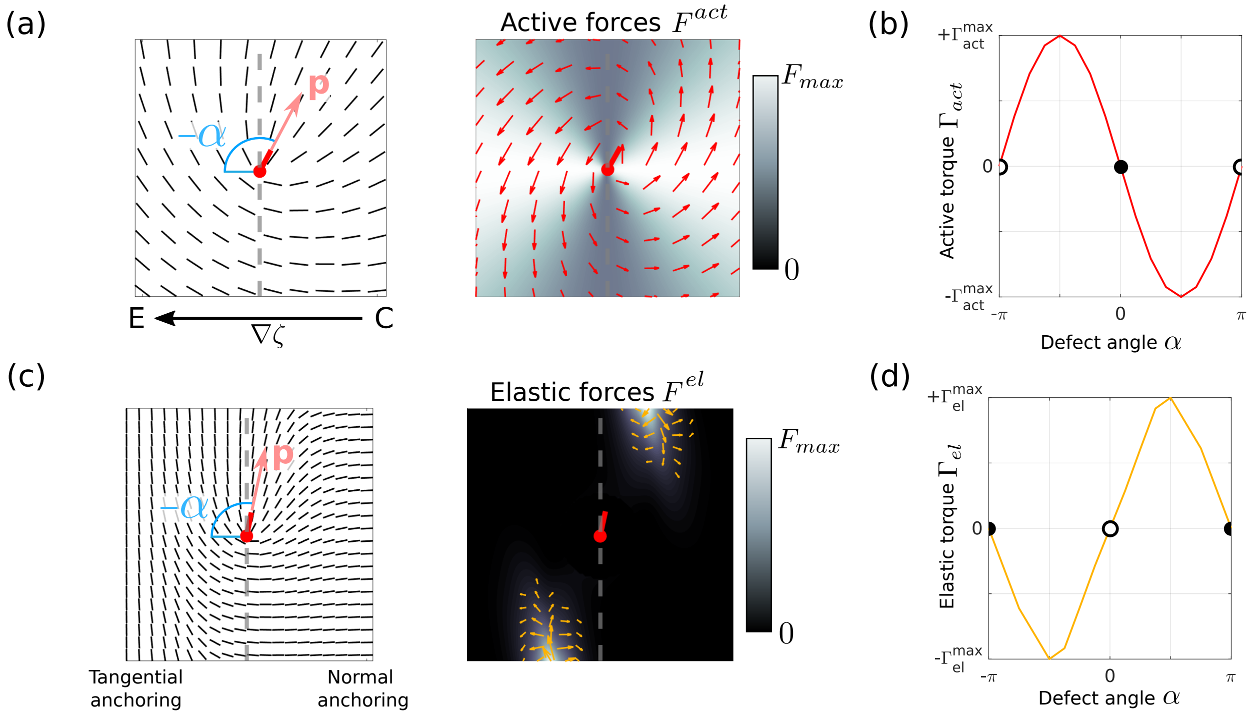


FIG. S3: (a) Director field (left) and active forces (right) of a +1/2 defect with orientation $\mathbf{p}$ at a finite angle $\alpha$ with respect to an activity gradient $\nabla\zeta$ (negative sign indicates clockwise rotation). (b) Active forces $F^{act}$ create a torque $\Gamma_{act} \sim \mathbf{p} \times \nabla\zeta$ on the defect, which reaches a maximum at $\alpha = \pm\pi/2$ and vanishes for $\alpha = 0, \pi$. Active torques thus align +1/2 defects parallel to activity gradients, which is evident from the stable fixed-point at $\alpha = 0$. The magnitude of active torque $\Gamma^{max}_{act}$ depends on the specific activity profile in the vicinity of defects, but generally scales with the magnitude of activity gradients, $\Gamma^{max}_{act} \sim \zeta_{max}$. (c) Director field (left) and elastic forces (right) of a +1/2 defect with orientation $\mathbf{p}$ at a finite angle $\alpha$ with respect to planar boundary conditions set up by the effective anchoring force, favouring normal anchoring on the contractile side and tangential anchoring on the extensile side of activity interfaces. (d) Elastic forces $F^{el}$, which are strongest at points of large bend or splay distortions, create an elastic torque $\Gamma_{el}$ on the defect, which reaches a maximum at $\alpha = \pm\pi/2$ and gives rise to a stable fixed point at $\alpha = \pi$. Elastic forces thus align +1/2 defects anti-parallel to activity gradients. The magnitude of elastic torque $\Gamma^{max}_{el}$ depends on the specific distortion profile around defects, but generally scales with the magnitude of the elastic energy $f_{el}$, $\Gamma^{max}_{el} \sim K_{el}$. Active and elastic forces were calculated from $\Pi^{act}$ and $\Pi^{el}$, respectively, using a fixed director field $\mathbf{Q}$ on a 2D lattice of size $100 \times 100$.

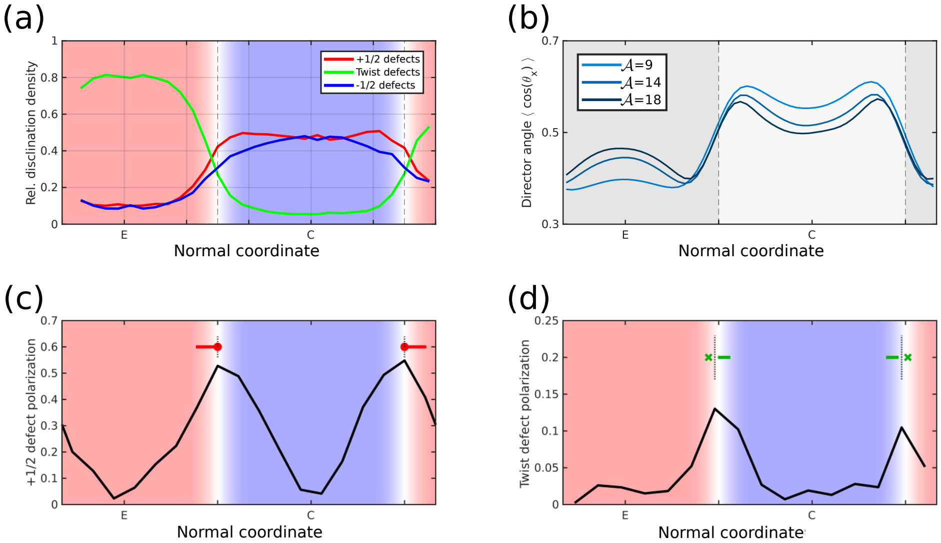


FIG. S4: Sharp activity interfaces in 3D systems give rise to qualitatively similar dynamics as sinusoidal activity variations. (a) The relative density of $\pm 1/2$ and twist disclination and (b) the average director field alignment directly follow the spatial variations in active stress. (c,d) $+1/2$ defects and twist defects are strongly polarized at active interfaces and show no polarization in bulk regions.

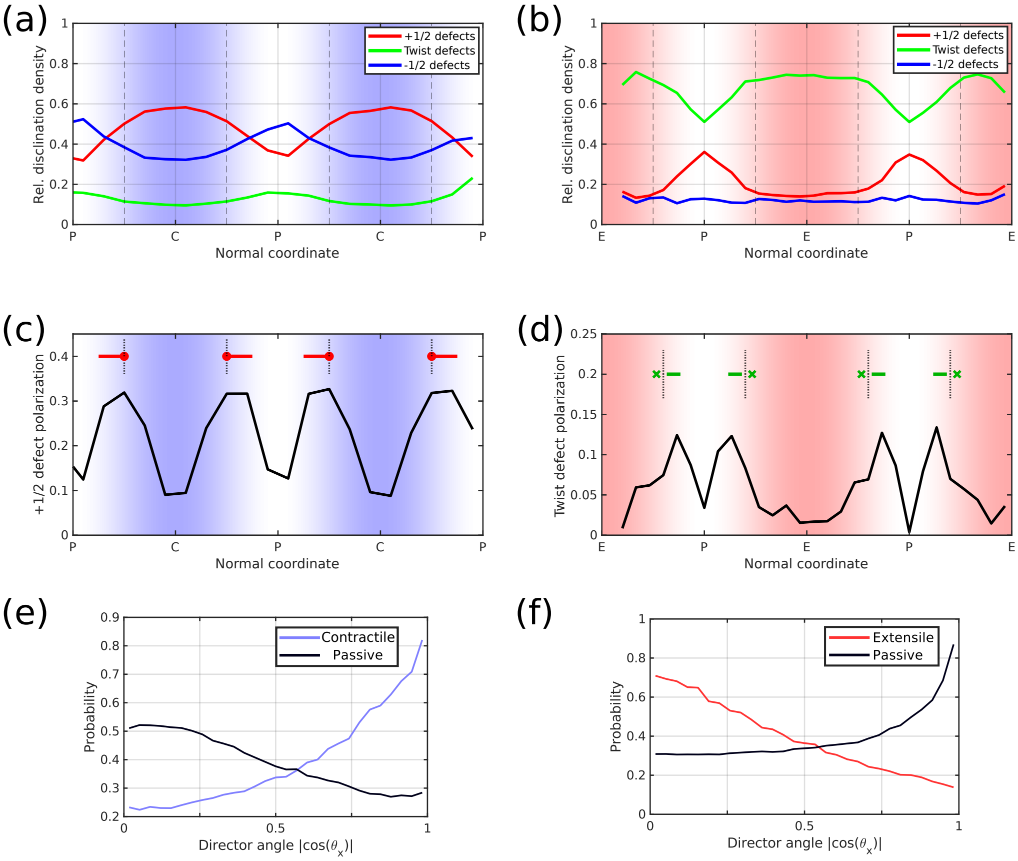


FIG. S5: (a,c) Three-dimensional systems featuring contractile-passive domains, $\zeta(\mathbf{x}) = \zeta_{max}(\cos(\mathbf{k}\cdot\mathbf{x}) - 1)$, are dominated by passive $-1/2$ and motile $+1/2$ disclination line segments, which are polarized in the same direction as in extensile-contractile systems. (e) The time-averaged distribution of the director field in the turbulent regime shows significant normal alignment with respect to the gradient direction in contractile regions and tangential alignment in passive domains. (b,d) Extensile-passive systems with $\zeta(\mathbf{x}) = \zeta_{max}(\cos(\mathbf{k}\cdot\mathbf{x}) + 1)$ contain predominantly twist segments which are polarized at points of large activity gradients and point towards passive domains. (f) The director field shows tangential alignment with respect to the gradient direction in extensile domains and normal alignment in passive domains.

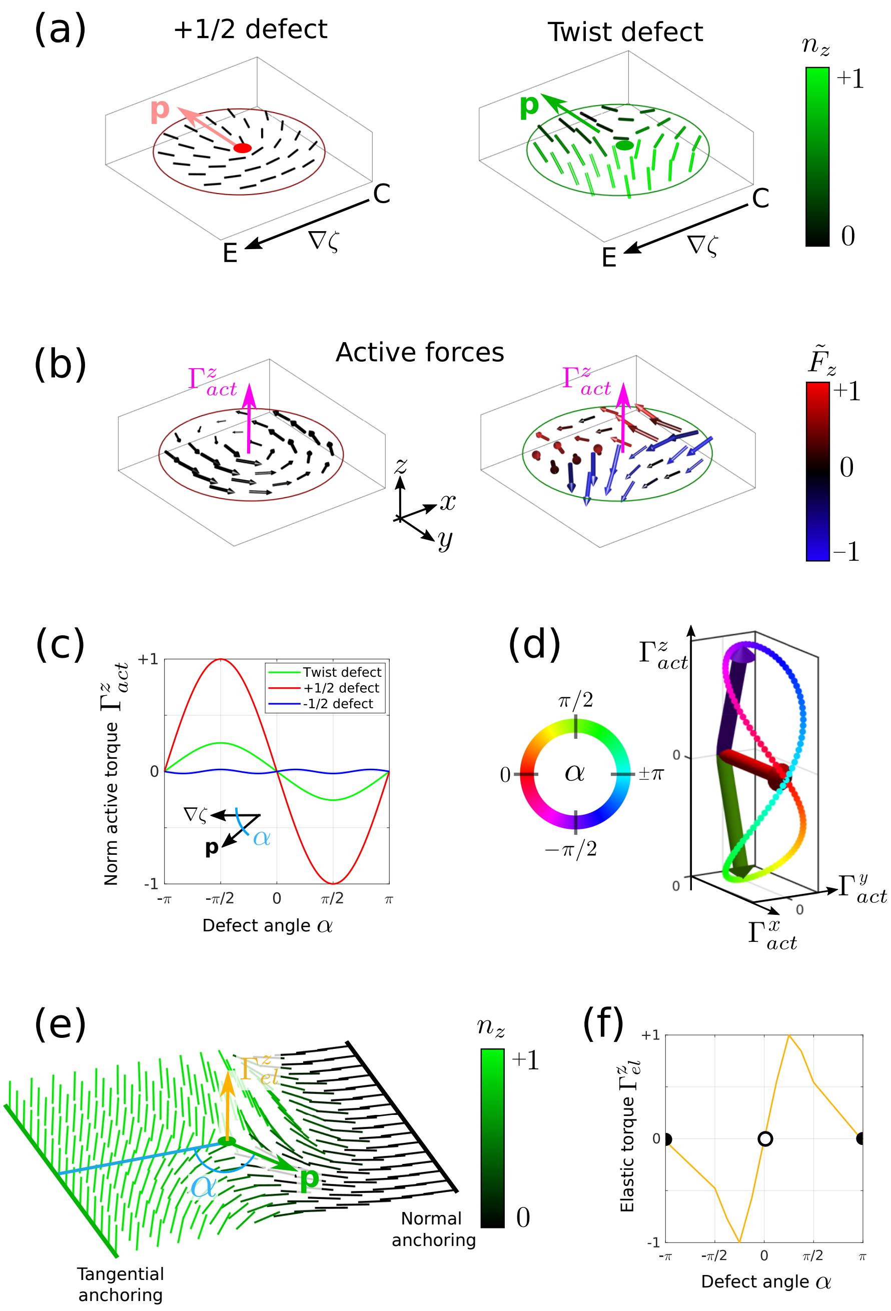


FIG. S6: (a) Director fields of a $+1/2$ (left) and radial twist disclination (right) with orientation $\mathbf{p}$ and an applied activity gradient $\nabla\zeta$. While $+1/2$ disclinations are quasi-2D, the director field around twist disclinations features out-of-plane components $n_z$. (b) Active forces around $+1/2$ disclinations (black arrows) are confined to the defect plane ($xy$) and produce a torque $\Gamma_{act} \sim \mathbf{p} \times \nabla\zeta$ along the $z$-axis (pink arrow), which rotates the defect orientation $\mathbf{p}$. Active forces around twist disclinations feature out-of-plane components $F_z$ (see colorbar), creating an active torque $\Gamma_{act}$ which does not strictly point along the $z$-axis. The in-plane defect orientation $\mathbf{p}$ is only affected by component $\Gamma^z_{act}$, while components $\Gamma^x_{act}$ and $\Gamma^y_{act}$ change the overall direction of the defect line. (c) Active torque $\Gamma^z_{act}$ as a function of angle $\alpha$ between defect direction $\mathbf{p}$ and activity gradient $\nabla\zeta$ for different defect types. Like in 2D, active torques align defect orientations $\mathbf{p}$ parallel to activity gradients ($\alpha = 0$). The orientation $\mathbf{p}$ of twist defects, however, is much less affected by active torques compared to $+1/2$ defects. (d) The active torque vector $\Gamma_{act}$ on twist defects changes direction as a function of defect angle $\alpha$. The magnitude of the $z$-component $\Gamma^z_{act}$ reaches a maximum for $\alpha = \pm\pi/2$, while the out-of-plane component $\Gamma^x_{act}$, which points along the gradient direction, peaks at $\alpha = 0, \pi$, where its sign depends on the chirality of the twist defect. (e) Director field of of a twist defect with orientation $\mathbf{p}$ at a finite angle $\alpha$ with respect to boundary conditions set up by the effective anchoring force, favouring normal and tangential anchoring on the contractile and extensile side, respectively. (f) Elastic forces in the defect plane create an elastic torque $\Gamma^z_{el}$ which aligns twist defects anti-parallel to activity gradients. Active and elastic forces were calculated from $\Pi^{act}$ and $\Pi^{el}$, respectively, using a fixed director field $\mathbf{Q}$ on a 3D lattice of size $100 \times 100 \times 20$.
